# Supplementary material for: Online learning in MDPs with linear function approximation and bandit feedback
Source: arXiv:2007.01612 source file (2021-06-12)
Supplement: Supplementary file 1 [file appendixC.tex]

\section{Proof of Theorem~\ref{th_improved}}
\label{appendixC}
The improvement in the regret bound comes from applying an importance-weighting trick in the proof of Lemma~\ref{quadratic} to bound the problematic term 
$\textup{tr}\bpa{\Sigma_{h}^*\Sigma_{t,h}^{-1}}$. Specifically, we write
\begin{align*}
 \textup{tr}\bpa{\Sigma_{h}^*\Sigma_{t,h}^{-1}} &= \trace{\EEt{ \varphi(\tX, \pi_t(\tX))\varphi(\tX, \pi_t(\tX))\transpose}\Sigma_{t,h}^{-1}}
 \\
 &= \trace{\EEt{\frac{f^*_h(X_{t,h})}{f_h^{\pi_t}(X_{t,h})}  \varphi(X_{t,h}, \pi_t(X_{t,h}))\varphi(X_{t,h}, \pi_t(X_{t,h}))\transpose}\Sigma_{t,h}^{-1}}
 \\
 &\le \rho \cdot \trace{\EEt{\varphi(X_{t,h}, \pi_t(X_{t,h}))\varphi(X_{t,h}, \pi_t(X_{t,h}))\transpose}\Sigma_{t,h}^{-1}} = \rho d,
\end{align*}
where we used our assumption on the likelihood ratio in the inequality. Using this bound instead of the one in Equation~\eqref{eq:quadratic_final} at the end of the proof of Lemma~\ref{quadratic} yields the improved bound
\[
\EEt{\sum_{a=1}^K    \pi_t(a|\tX)   \biprod{\varphi(\tX, a)}{\htheta_{t,h}}^2} \le  (H-h)^2 d\pa{\frac{ 1}{3} + \rho }.
\]
The proof of Theorem~\ref{th_improved} is then concluded similarly as the proof of Theorem~\ref{th_regret}.

\jmlrQED

\subsection{Complete regret bound on Theorem~\ref{th_improved}.}\label{app:full_bound_improved}
 For  $\gamma\in (0,1)$, $M \ge 0$, any positive $\eta \le \frac{2}{(M+1) H}$ and any positive $\beta \le \frac{1}{2\sigma^2}$, the expected 
regret of \linexprl  over $T$ episodes, satisfies
\begin{align*}
	R_T \le& 2T \sigma R H\cdot \exp\pa{-\gamma\beta\lambdamin M} + \gamma  H^2 T + \eta H^3 d\pa{  \frac{ 1}{3} +  \rho}T  + H \cdot \frac{\log K}{\eta}.
\end{align*}
Furthermore, letting $\beta = \frac{1}{2\sigma^2}$, $M = \left\lceil\frac{ \sigma^2 \log (T 
	\sigma^2 R^2)}{\gamma  \lambdamin}\right\rceil$, $\eta =\frac 1H \sqrt{\frac{\log K }{T d \rho}}$, $\gamma = 
\sqrt{\frac{d \rho \log K }{T} }$ and supposing that $T$ is large enough so that the above constraints are satisfied, we 
also have 
\begin{align*}
	R_T \le& 3 H^2 \cdot\sqrt{T d  \rho \log K  }+ \frac{1}{3}H^2 \sqrt{\frac{T d  \log K}{\rho } }  + 4H\sqrt{T}.
\end{align*}
